# Supplementary material for: Structured Sparsity: Discrete and Convex approaches
Source: arXiv:1507.05367 source file (2015-07-20)
Supplement: Supplementary file 1 [file appendix.tex]

\section{Appendix}

\subsection{Case study: discrete vs.\ convex interpretability}
\label{sec:discrete_vs_convex}

The following stylized example illustrates situations that can potentially be encountered in practice. 
In these cases, the group-support obtained by the convex relaxation will not coincide with the discrete definition of group-cover, while the dynamical programming algorithm of Prop.~\ref{prop:DP1} is able to recover the correct group-cover.

Let $\N = \{1, \ldots, 11\}$ and let $\GG = \{\G_1 = \{1, \ldots, 5\},~\G_2 = \{4, \ldots, 8\},~\G_3 = \{7, \ldots, 11\}\}$ be the loopless pairwise overlapping groups structure with $3$ groups of equal cardinality. Its group graph is represented in Fig.~\ref{fig:example}. 
Consider the $2$-group sparse signal ${\bf x} = [0~0~1~1~1~0~1~1~1~0~0]^\top$, with minimal group-cover $\mathcal{M}({\bf x}) = \{\G_1, \G_3\}$. 

\tikzstyle{place}=[circle,draw=black,fill=white,thick, minimum size=6pt, inner sep=0pt]
\begin{figure}
\centering
\begin{tikzpicture}[-,>=stealth',shorten >=1pt,auto,node distance=1.5cm, semithick]
	\node[place] (n1) at (0,0)    [label=below:$\G_1$] {};% = \{1, 2, 3\}$};
	\node[place] (n2) at (1.5,1) [label=above:$\G_2$] {};% = \{1, 2, 3\}$};
	\node[place] (n3) at (3,0)    [label=below:$\G_3$] {};% = \{1, 2, 3\}$}
	
\draw (n1) to node {$\{4,5\}$} (n2);
\draw (n2) to node {} (n1);
\draw (n2) to node {$\{7,8\}$} (n3);
\draw (n3) to node {} (n2);
\end{tikzpicture}
\caption{\label{fig:example} The group-graph for the example in Section~\ref{sec:discrete_vs_convex}}
\end{figure}

The dynamic program of Prop. \ref{prop:DP1}, with group budget $G = 2$, correctly identifies the groups $\G_1$ and $\G_3$. 
The TU linear program \eqref{eq:PR}, with $0 <  \lambda \leq 2$, also yields the correct group-cover.
Conversely, the decomposition obtained via \eqref{eq:atomic_norm} with unitary weights is unique, but is not group sparse. In fact, we have $\mathcal{S}({\bf x}) = \breve{\mathcal{S}}({\bf x}) = \GG$.
We can only obtain the correct group-cover if we use the weights $[1~d~1]$ with $d > \frac{2}{\sqrt{3}}$, that is knowing beforehand that $\G_2$ is irrelevant.
\begin{rem}
Indeed, if the convex relaxation always recovered the correct minimal group-cover, it would be possible to solve the discrete NP-hard problem in polynomial time.
\end{rem}
